# Supplementary material for: LEGOStore: A Linearizable Geo-Distributed Store Combining Replication and Erasure Coding
Source: arXiv:2111.12009 source file (2022-07-04)
Supplement: Supplementary file 1 [file optimized_get.tex]

\section{Protocol Optimizations}
\label{sec:protocol-opt}

\begin{figure}[]
\begin{mdframed}
\textbf{Optimized\_get in ABD algorithm}:
\footnotesize
\medskip

% \underline{\textit{get-timestamp-value}}: Send \textit{get-timestamp-value} message to all servers, and wait for all of them to respond with (\textit{tag}, \textit{value}). On receiving response, if all the responses are for the same version, then return to client the \textit{value}. Otherwise, select the largest timestamp and its corresponding value (\textit{max-tag}, \textit{max-value}).

% \medskip

% \underline{\textit{\textit{put-value}}}: Send \textit{put-value} message with (\textit{max-tag}, \textit{max-value}) to the write quorum and wait for all of them to respond. Return \textit{max-value} to client.

\underline{\textit{get-timestamp-value}}: Send \textit{get-timestamp-value} message to \textit{max}(\textit{q1}, \textit{q2}) number of servers, and wait for all of them to respond with (\textit{tag}, \textit{value}). Let $t*$ be the pair with the maximum value. If at least \textit{q2} number of responses have the same tag as $t*$, then return to client with the \textit{value} of $t*$. Otherwise, go to the next phase.

\medskip

\underline{\textit{\textit{put-value}}}: Send \textit{put-value} message with $t*$ to the \textit{q2} number of servers and wait for all of them to acknowledge. Return \textit{value} of $t*$ to client.

\end{mdframed}
\caption{Client side optimistic GET requests for ABD}
\label{opt_get_label}
\end{figure}

\begin{figure}[]
\begin{mdframed}
\textbf{Optimized\_get in CAS algorithm}:
\footnotesize
\medskip

% \underline{\textit{get-timestamp-value}}: Send \textit{get-timestamp-value} message to all servers, and wait for all of them to respond with (\textit{tag}, \textit{value}). On receiving response, if all the responses are for the same version, then return to client the \textit{value}. Otherwise, select the largest timestamp and its corresponding value (\textit{max-tag}, \textit{max-value}).

% \medskip

% \underline{\textit{\textit{put-value}}}: Send \textit{put-value} message with (\textit{max-tag}, \textit{max-value}) to the write quorum and wait for all of them to respond. Return \textit{max-value} to client.

\underline{\textit{get-timestamp-value}}: Send \textit{get-timestamp} message to \textit{max}(\textit{q1}, \textit{q4}) number of servers, and wait for all of them to respond with \textit{tag}. Let $t*$ be the maximum tag. If at least \textit{q4} number of responses are for the same tag as $t*$ and a value with $t*$ is available in the local cache, then return to client with the \textit{value} in the cache. Otherwise, go to the next phase.

\medskip

\underline{\textit{\textit{put-value}}}: Send \textit{put-value} message with $t*$ to \textit{q4} number of servers and wait for each \textit{server$_{i}$} to respond with ($t*$, \textit{chunk$_{i}$}). Decode the chunks with Reed-Solomon algorithm to retrieve the \textit{value}. Add \textit{value} to the cache. Return \textit{value} to client.

\end{mdframed}
\caption{Client side optimistic GET requests for CAS}
\label{opt_get_label}
\end{figure}
After each read operation, we need to make sure that \textit{q2} number of servers has a tag the same as tag of the read operation or a bigger tag, for ABD, or \textit{q4} number of servers has that tag flagged \textit{FIN} for CAS.

By using some gossip messages among servers, we can make sure more servers has the tuple of max timestamp and increase the change of doing get operations in one phase.

There are two possibilities, (a) \textit{q1} $\geq$ \textit{q2} for ABD or \textit{q1} $\geq$ \textit{q4} for CAS; and (b) \textit{q1} $<$ \textit{q2} for ABD or \textit{q1} $<$ \textit{q4} for CAS. In case (a), since we have received the timestamps from \textit{q1}, and all of them are equal, it means at least \textit{q2} number of servers has the timestamp in the case of ABD and it suffices. In the case of CAS, it can be inferred that at least \textit{q4} number of servers has the tag flagged \textit{FIN}. In case (b), we should send requests to \textit{q2} and \textit{q4} in ABD and CAS respectively instead of \textit{q1}. Please note that, this change does not affect the algorithms because \textit{q2} and \textit{q4} are bigger than \textit{q1} which means we can safely ignore (\textit{q2} - \textit{q1}) for ABD or (\textit{q4} - \textit{q1}) for CAS, and do the regular two phase get. However, if all the received responses are equal, it means there is at least \textit{q2} and \textit{q4} number of the timestamp in the system.
