# Supplementary material for: LEGOStore: A Linearizable Geo-Distributed Store Combining Replication and Erasure Coding
Source: arXiv:2111.12009 source file (2022-07-04)
Supplement: Supplementary file 10 [file optimized_get_analysis.tex]

\section{Analysis of Optimized GET Fraction}

A GET operation can be done in one phase\footnote{Reducing both latency and cost} if all the received timestamps in from the the servers in quorum Q1 are equal. In our analysis, we try to answer to these two questions: 1) what is the fraction of optimized GETs that clients on datacenter $s$ experience if we assume there is no concurrent operations?, and 2) what is the impact of concurrent operations from the clients that uses the same set of quorums on the fraction of optimized GET that clients on datacenter $s$ experience?

The answer to the first question can help us to estimate the fraction of optimized GET. Second question helps us justify the interesting result that pairwise latency affects the fraction of optimized GET.

\subsection{Optimized GET Fraction Without Concurrency}
\label{sec:opt-get-seq}
In this section, we assume all the operations happen sequentially, and we are interested to compute the fraction of optimized GET for a client in one data center that uses $Q_1$ and $Q_2$. The condition to have one-phase GET will be that previous operations happen such that all the servers in $Q_1$ have the same timestamp.

First, we examine one simple example both theoretically and through experiments. Then, we try to extend our formulation.

We consider a case where we have a uniform client distribution among all the 9 data centers\footnote{we assign each data center an ID from 1 to 9. Each data center is running a server to serve the operation as well.}. Clients on data centers 1 to 5 and 7, called group 1, are using $Q_1={3, 6}$ and $Q_2={3, 6}$ to do operations, and clients on other data centers (6, 8, and 9), called group 2, are using $Q_1={6, 9}$ and $Q_2={6, 9}$. We assume the read ratio is 50\%. We want to compute the probability of the GET operation, called $o_1$ that is being done by a client from group 1, being optimized GET. Let $o'_1$ be the last operation before $o_1$ done by a client in group 1. If all the operations between $o_1$ and $o'_1$ are read operations, $o_1$ is optimized GET.

\noindent To compute the probability, we have:
\begin{equation}
% \begin{split}
\begin{aligned}
\label{eq:seq-opt-get-ex}
 p_{(o'_1 \text{ is from group 1})} &= \frac{\text{\# data centers in group 1}}{\text{Total \# data centers}} = \frac{6}{9} \\
 P_{(o \text{ is GET})} &= read\_ratio = \frac{1}{2} \\
 P_{(o_1 \text{ is optimized GET})} &= \frac{6}{9} + ((1 - \frac{6}{9}) \cdot \frac{1}{2}) \cdot \frac{6}{9} + ((1 - \frac{6}{9}) \cdot \frac{1}{2})^{2} \cdot \frac{6}{9} + ... \\
 &= \frac{2}{3} \cdot \sum\limits_{i=0}^\infty \Big( (1-\frac{2}{3}) \cdot \frac{1}{2} \Big)^i = 0.8
\end{aligned}
% \end{split}
\end{equation}

With the same approach we can compute the same probability for clients from group 2 as $P_{o_2 \text{ is optimized get}} = 0.5$ where $o_2$ is a read operation from group 2.

Table~\ref{tab:exp-opt-get} is showing the fraction of optimized GET that clients from each data center could achieve. The results are consistent.

\begin{table}
\centering
\caption{Experimental fraction of GET operation that could be done in one phase from each data center. Please note in this experiment the arrival rate is 9 request per second, so we can assume the operations are sequential.}
\label{tab:exp-opt-get}
\begin{tabular}{|c|c|c|c|} 
\hline
\rowcolor[rgb]{0.851,0.851,1} \begin{tabular}[c]{@{}>{\cellcolor[rgb]{0.851,0.851,1}}c@{}}\textbf{Data}\\\textbf{center ID}\end{tabular} & \begin{tabular}[c]{@{}>{\cellcolor[rgb]{0.851,0.851,1}}c@{}}\textbf{Fraction of}\\\textbf{Optimized GET}\end{tabular} & \begin{tabular}[c]{@{}>{\cellcolor[rgb]{0.851,0.851,1}}c@{}}\textbf{Data}\\\textbf{center ID}\end{tabular} & \begin{tabular}[c]{@{}>{\cellcolor[rgb]{0.851,0.851,1}}c@{}}\textbf{Fraction of}\\\textbf{Optimized GET}\end{tabular} \\ 
\hline \hline
1 & 0.77 & 6 & 0.46 \\ 
\hline
2 & 0.79 & 7 & 0.75 \\ 
\hline
3 & 0.75 & 8 & 0.48 \\ 
\hline
4 & 0.75 & 9 & 0.51 \\ 
\hline
5 & 0.78 & - & - \\
\hline
\end{tabular}
\end{table}

A read operation $o_i$ from a client on data center $i$, that uses $Q_{i,1}$, can be done in one-phase if all the received timestamps are equal. Thus, to compute the probability of $o_i$ being optimized GET, we need to compute the probability of every sequence of the operations that make the timestamps on the servers in $Q_{i,1}$ equal, and sum them up. 

\todo{There is a problem in this generalization where the middle read operations can be done in one phase!}

$k$ is the number of read operations between the last write operation and $o_i$. The probability of the read operation $o_i$ being optimized GET is equal to: 

\begin{equation}
% \begin{split}
\begin{aligned}
\label{eq:seq-opt-get}
&\sum\limits_{k=0}^\infty P_{(A(k))} \\
&\text{Where A(k) is the sequence of operations that:} \\
&\text{a) starts with a write operation, and} \\
&\text{b) }Q_{i, 1} \subseteq \cup_{j=0}^{k} Q_{DC(j),2} \text{operation $j$th has been done by DC(j)}
\end{aligned}
% \end{split}
\end{equation}

\subsection{Optimized GET Fraction With Concurrency}
Surprisingly, pairwise latencies among clients and servers play an important role in fraction of optimized GET.

We demonstrate this finding through an example. First, we try to justify our finding theoretically, and then we use our prototype to gather the experimental results.

We use the same example as in Section~\ref{sec:opt-get-seq} but we increase the arrival rate to 100 requests per second to increase concurrency.

One event that could prohibit optimized GET is that a concurrent write operation, using the same quorum set, happens, and the write operation updates the timestamp on at least one of the servers in Q1 but not all of them before the GET operation receives the timestamp.

For example, in Figure~\ref{fig:opt-get1}, the client on DC 1 is doing the first phase of a GET operation, and the client on DC 2 is doing the second phase of a write operation. The upwards arrows are requests from the clients and the downward arrows are responses. the client on DC 2 has only updated s5 before the server responds to the other client’s request, so the client on DC 1 will receive two different timestamps and the GET operation can not be optimized.

\begin{figure}
    \includegraphics[width=\columnwidth]{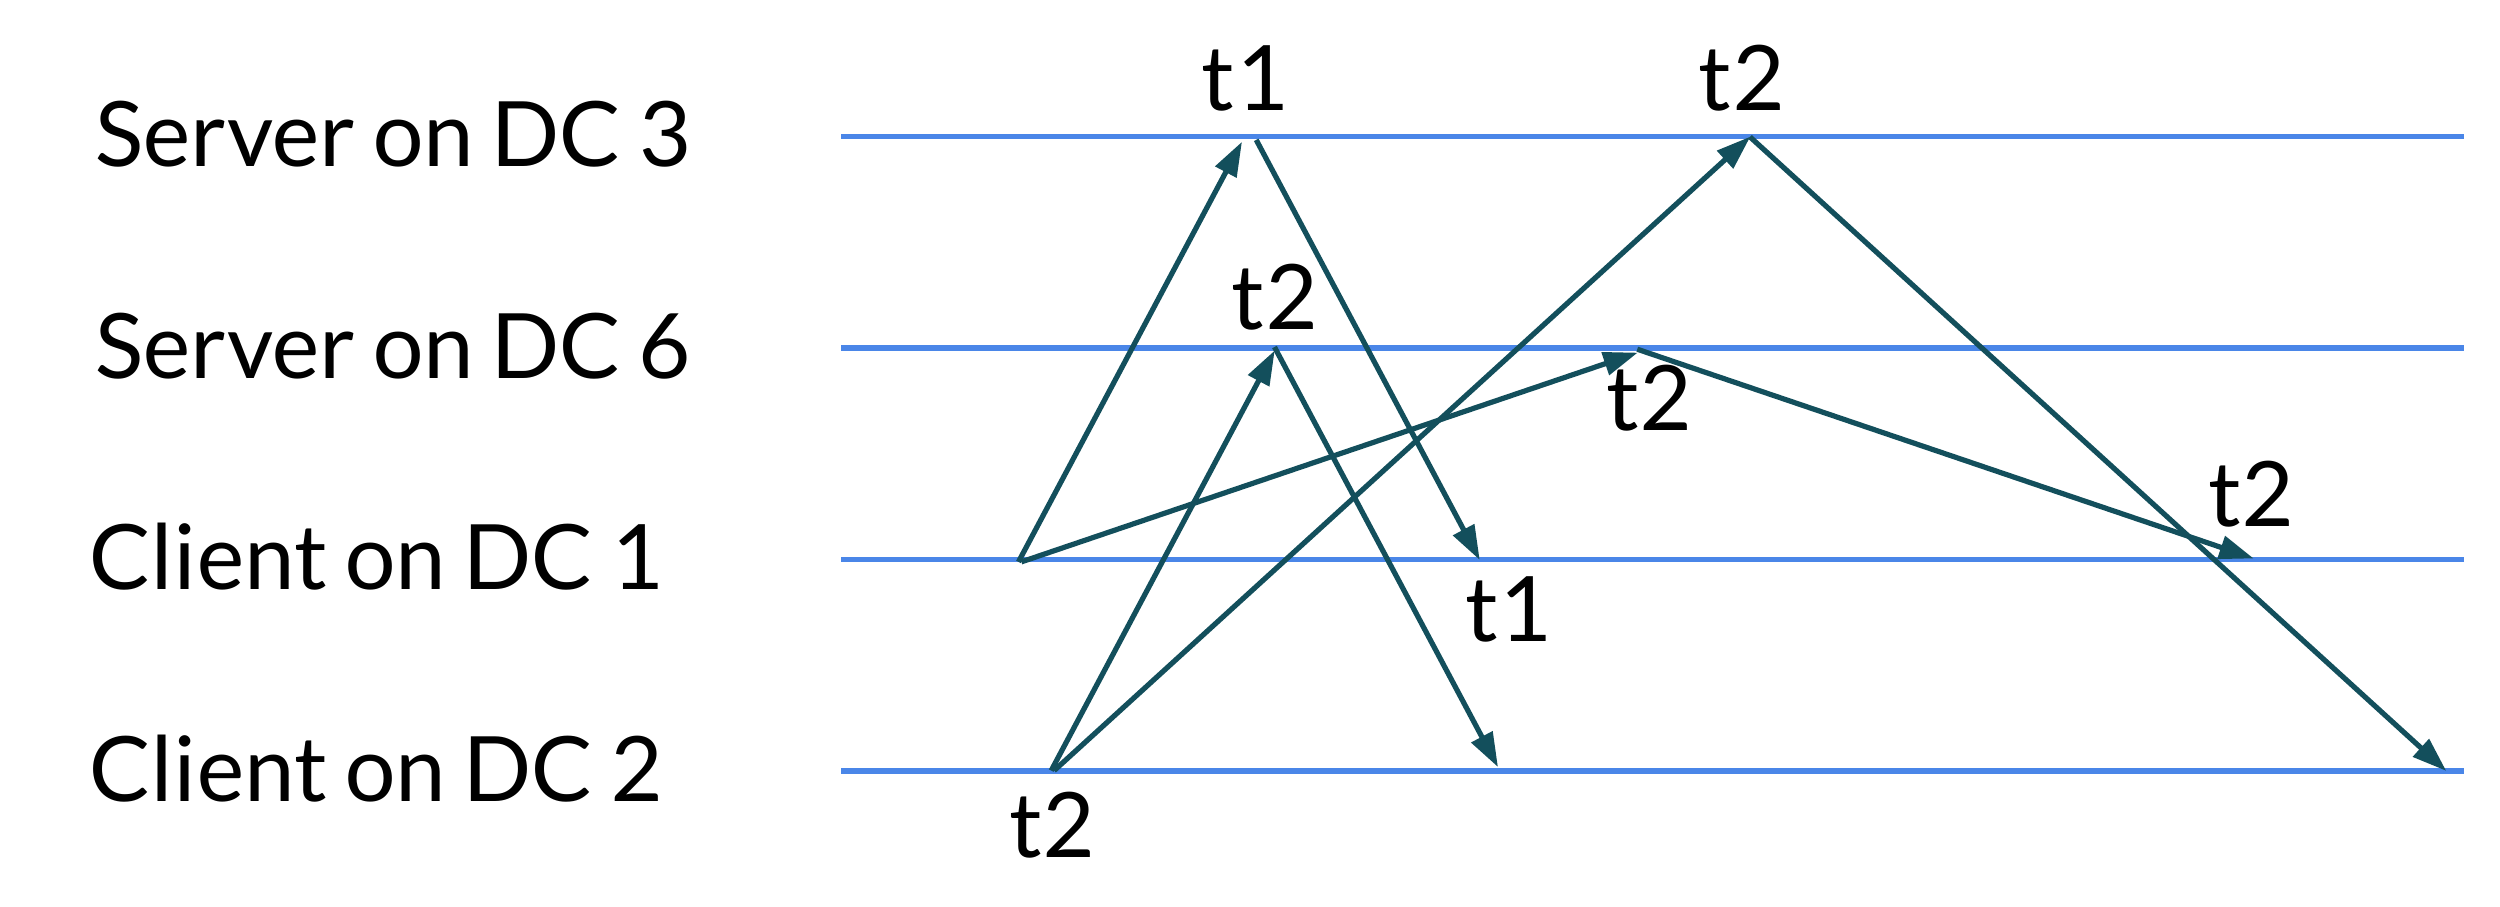}
    \caption{Messages for the phase 1 of a read operation by the client on DC 1 and messages for the phase 2 of a write operation by the client on DC 2.}
    \label{fig:opt-get1}
\end{figure}

The probability of such an event depends on clients from which DCs are committing the write and read operations.  For example, in Figure~\ref{fig:opt-get2}, the write operation is concurrent with the read operation, but it does not hinder the read operation from being optimized.

\begin{figure}
    \includegraphics[width=\columnwidth]{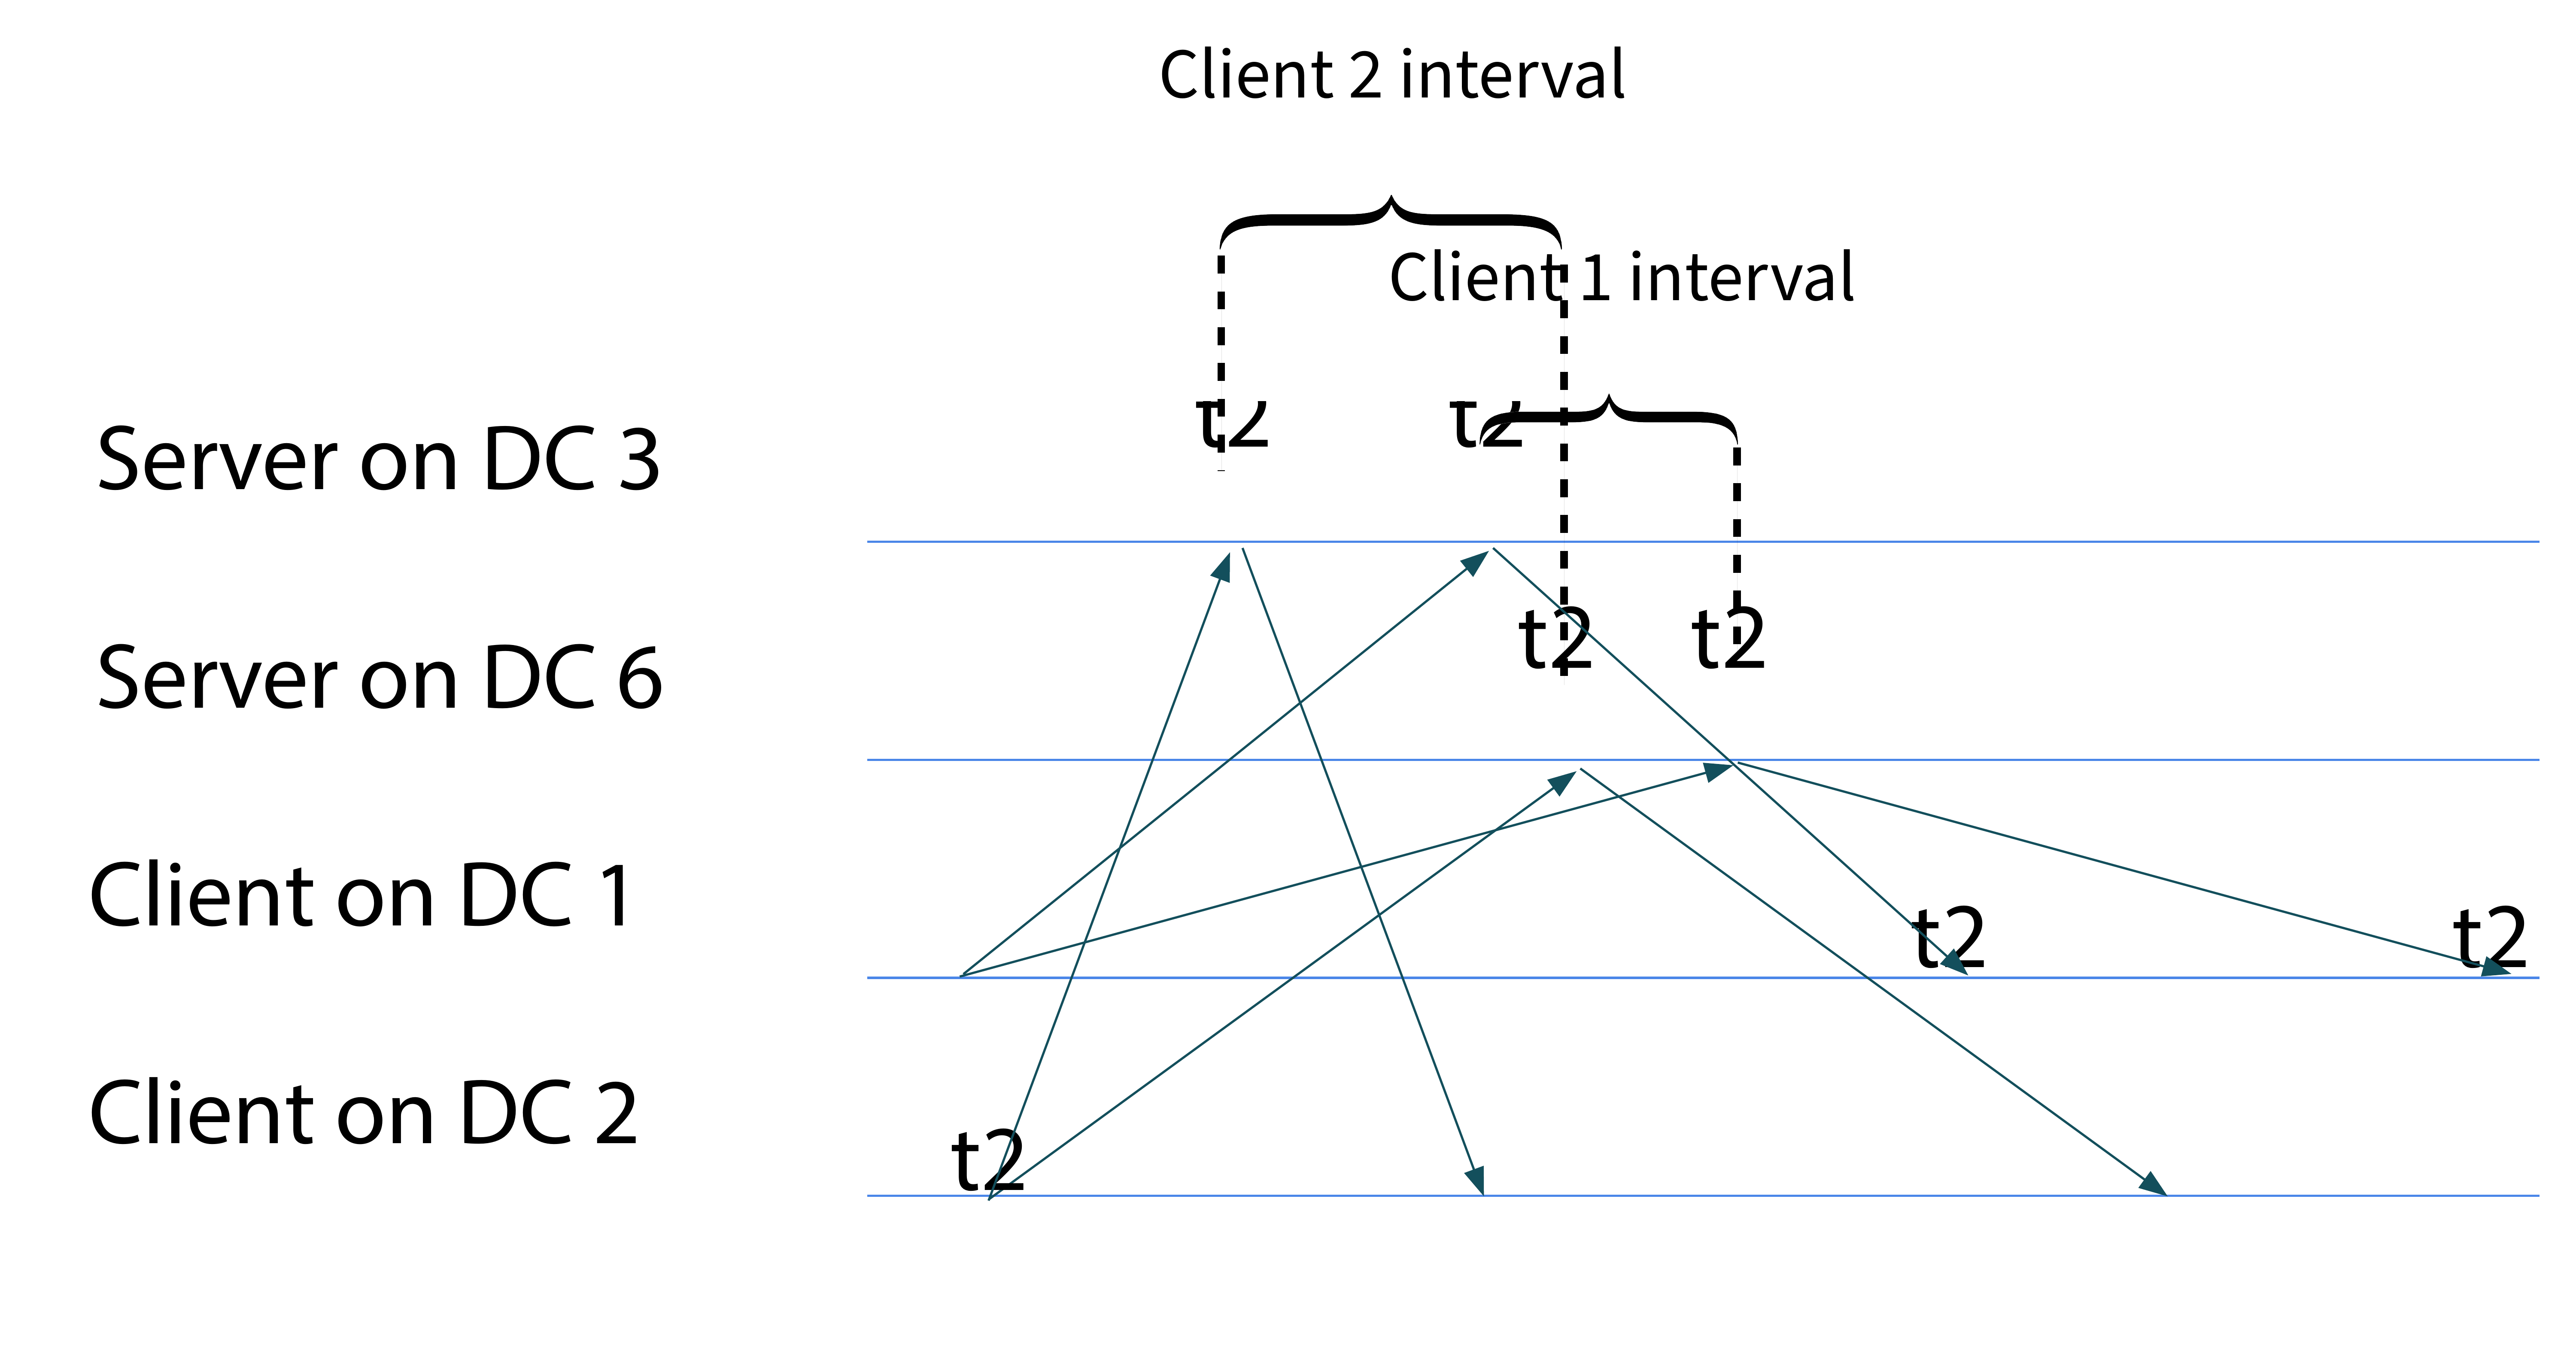}
    \caption{Messages for the phase 1 of a read operation by the client on DC 1 and messages for the phase 2 of a write operation by the client on DC 2.}
    \label{fig:opt-get2}
\end{figure}

Therefore, the interval that no write operations should happen on DC 2 so the GET operation on DC 1 receives the same timestamps is $|\text{Client 1 interval} - \text{Client 2 interval}|$. And, if the clients reach the servers in the opposite order, the interval will be $(\text{Client 1 interval} + \text{Client 2 interval})$.

We have pairwise latencies among datacenters and by dividing those by 2, we approximate the latencies of reaching other datacenters. And, by using the mentioned formula, we compute the intervals. For example, we compute the intervals during which no write operations should happen on datacenters so that a GET operation on s0 can be done in one phase.

The following table is showing the difference between latencies reaching s2 and s5. A negative number means it reaches s5 sooner and a positive number means it reaches s2 sooner.
